# Supplementary material for: TigerLily: Finding drug interactions in silico with the Graph
Source: arXiv:2204.08206 source file (2022-04-18)
Supplement: Supplementary file 1 [file appendix.tex]

\appendix

\section{Multi-scale node representations}
